# Supplementary material for: Habit learning is associated with efficiently controlled network dynamics in naive macaque monkeys
Source: arXiv:2511.10757 ancillary file (2025-11-13)
Supplement: Supplementary file 1 [file 2025_nct_habit_learning_supplement.pdf]

# SUPPLEMENTARY MATERIAL: Habit learning is associated with efficiently controlled network dynamics in naive macaque monkeys

Julia K. Brynildsen[1,†], Panagiotis Fotiadis[1,2,†], Karol P. Szymula[1,3,4,†], Jason Z. Kim[1,5], Fabio Pasqualetti[6], Ann M. Graybiel[7,8], Theresa M. Desrochers[9,‡,*], and Dani S. Bassett[1,10,11,12,13,14,‡,*]

[1]Department of Bioengineering, School of Engineering & Applied Science, University of Pennsylvania, Philadelphia, PA 19104 USA

[2]Department of Neuroscience, Perelman School of Medicine, University of Pennsylvania, Philadelphia, PA 19104, USA

[3]Department of Biomedical Engineering, University of Rochester, Rochester, NY 14642 USA

[4]Medical Scientist Training Program, University of Rochester School of Medicine and Dentistry, Rochester, New York, USA

[5]Department of Physics, Cornell University, Ithaca, NY, 14853, USA

[6]Department of Mechanical Engineering, University of California, Riverside, CA 92521 USA

[7]McGovern Institute for Brain Research, Massachusetts Institute of Technology, Cambridge, MA 02139 USA

[8]Department of Brain and Cognitive Sciences, Massachusetts Institute of Technology, Cambridge, MA 02139 USA

[9]Department of Neuroscience, Department of Psychiatry and Human Behavior, Robert J. and Nancy D. Carney Institute for Brain Science, Brown University, Providence RI 02912 USA

[10]Department of Electrical & Systems Engineering, School of Engineering & Applied Science, University of Pennsylvania, Philadelphia, PA 19104 USA

[11]Department of Physics & Astronomy, College of Arts & Sciences, University of Pennsylvania, Philadelphia, PA 19104 USA

[12]Department of Neurology, Perelman School of Medicine, University of Pennsylvania, Philadelphia, PA 19104 USA

[13]Department of Psychiatry, Perelman School of Medicine, University of Pennsylvania, Philadelphia, PA 19104 USA

[14]Santa Fe Institute, Santa Fe, NM 87501 USA

[†]These three authors contributed equally.

[‡]These two authors contributed equally.

[*]Corresponding authors: theresa_desrochers@brown.edu; dsb@seas.upenn.edu

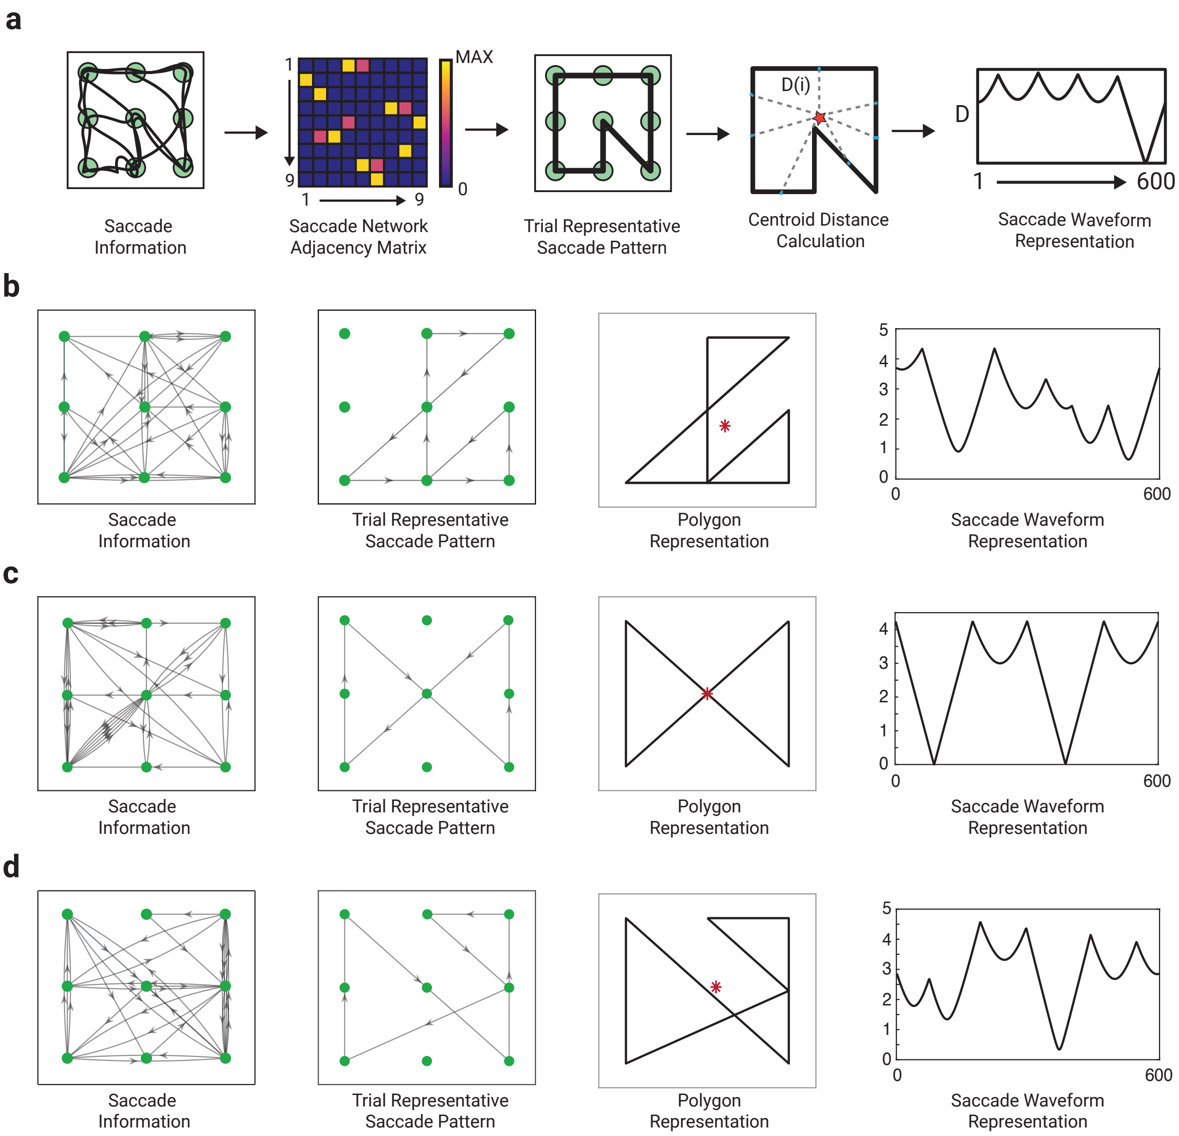


**Supplementary Figure 1: Classification of Trial Representative Saccade Patterns.** **(a)** Saccade information in the form of identified saccadic movements during a trial is collectively represented as an adjacency matrix, which in turn encodes a directed and weighted network. A total of nine nodes exist: one for every green target on the task grid. Edgeweights are calculated as the number of times that a saccade is made from one node to another. The network is converted into a trial representative saccade pattern by identifying the network cycle with the greatest sum of edge weights along its path. Each trial representative saccade pattern is treated as a 2-D polygon in the task grid space consisting of a set of (x,y) points. The saccade waveform is taken to be the vector of Euclidean distances between the polygon centroid and all of its points. A one dimensional interpolation is performed to reduce each saccade waveform to 600 values. **(b,c,d)** Example step-by-step classifications of saccade patterns from three randomly generated lists of saccades. The red star located on the polygon representations of the saccade patterns marks the centroid of the polygon.

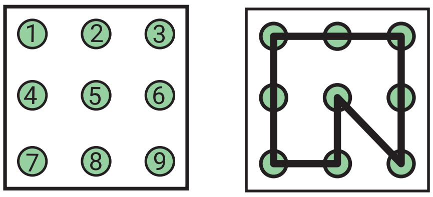


Grid Numbering     Example Pattern

**Example Numerical Representations**

(a) [1 3 6 9 5 8 7 1]

(b) [1 2 3 6 9 5 8 7 4 1]

(c) [1 3 9 5 8 7 1]

| #1-40 | #41-80 | #81-120 | #121-136 |
|---|---|---|---|
| [2 3 8 7 9 5 2] | [8 5 7 4 1 3 9 6 8] | [3 6 9 5 2 7 4 1 8 3] | [2 8 7 4 1 3 2] |
| [2 9 7 4 1 8 5 2] | [8 7 3 9 5 8] | [2 9 7 4 3 5 8 2] | [2 4 7 9 6 8 5 2] |
| [1 8 5 6 3 9 7 4 1] | [2 7 1 4 8 6 3 5 2] | [2 6 7 4 1 3 8 5 2] | [2 4 1 3 6 9 5 8 2] |
| [1 8 6 4 1] | [1 8 9 6 3 4 1] | **[1 3 9 8 7 4 1]** | [1 8 6 9 5 7 4 1] |
| **[2 3 9 8 7 4 1 5 2]** | [2 8 4 1 3 5 2] | [2 3 7 4 1 9 6 8 5 2] | [1 8 5 7 9 6 4 1] |
| [2 7 4 1 3 9 6 5 8 2] | [2 3 4 1 6 9 8 5 2] | [6 1 3 9 8 5 2 7 4 6] | [2 3 6 7 1 8 5 2] |
| [1 4 3 9 5 8 7 1] | [3 5 7 9 3] | **[5 8 5]** | [1 6 8 7 4 1] |
| [1 8 5 3 9 7 4 1] | [2 4 1 3 5 8 2] | [1 8 9 6 7 1] | [1 8 3 6 9 5 7 4 1] |
| [2 4 7 1 3 6 8 2] | [3 9 4 1 8 6 3] | [2 8 4 1 3 6 9 5 2] | [7 4 9 5 2 8 7] |
| [2 3 8 7 1 5 2] | [2 3 5 8 7 1 4 9 6 2] | **[2 3 9 7 4 1 8 2]** | [7 9 7] |
| [1 4 6 9 5 8 7 1] | [2 4 3 6 9 5 2] | [4 7 6 5 4] | [2 5 8 4 6 9 7 1 2] |
| [2 5 8 9 6 3 4 1 2] | [2 4 1 6 9 8 5 2] | [1 5 3 6 9 7 4 1] | [2 6 3 9 8 5 2] |
| [2 7 4 8 9 5 2] | [2 3 8 7 1 6 9 5 2] | [2 4 1 7 9 3 6 5 8 2] | [2 3 9 5 6 4 1 8 2] |
| [2 4 7 1 3 6 9 5 8 2] | [2 3 7 9 6 8 5 2] | [7 8 5 2 3 6 9 4 1 7] | [2 8 9 5 7 4 1 3 6 2] |
| [2 4 7 1 3 5 8 2] | [1 8 7 4 3 9 5 1] | [3 9 5 8 7 4 3] | [1 8 5 7 9 6 3 4 1] |
| [1 4 6 8 5 3 9 7 1] | [2 7 4 6 9 8 5 2] | [2 3 6 4 1 7 5 2] | [2 7 4 1 8 5 2] |
| [2 8 4 7 1 3 6 5 2] | [9 7 4 8 5 6 9] | [2 7 4 9 8 5 2] | |
| [2 8 7 9 5 2] | [1 6 9 7 1] | [2 7 1 3 6 5 8 2] | |
| [1 9 6 8 7 4 1] | [3 6 8 5 7 4 3] | [2 3 9 7 4 1 6 8 5 2] | |
| [2 5 7 4 1 9 6 3 8 2] | [2 3 9 6 7 4 1 8 5 2] | [2 9 7 5 2] | |
| [3 6 5 8 7 4 3] | **[4 8 5 2 3 6 9 7 4]** | [3 5 8 7 1 6 9 3] | |
| [1 8 7 9 6 4 1] | [2 6 5 8 7 4 1 3 2] | [2 4 7 1 6 9 3 5 8 2] | |
| [2 7 4 3 9 5 2] | [2 8 4 3 9 5 2] | [2 1 6 9 5 2] | |
| [3 7 4 1 9 3] | [2 8 7 4 1 9 2] | [1 9 5 8 7 4 1] | |
| [2 3 7 4 1 9 8 5 2] | [5 7 4 1 8 6 3 5] | [2 8 7 1 6 9 5 2] | |
| [2 3 9 7 1 5 8 2] | [1 8 5 9 6 7 4 1] | [2 3 6 4 8 5 2] | |
| [1 8 6 3 9 7 4 1] | [6 8 4 7 1 3 9 6] | [2 3 6 4 1 7 8 5 2] | |
| [2 3 7 4 1 8 5 2] | [2 8 7 4 1 6 5 2] | [2 3 7 4 1 6 9 8 5 2] | |
| [2 3 7 4 1 6 9 5 2] | [1 3 4 8 5 7 1] | [3 5 2 6 9 8 7 4 1 3] | |
| [9 7 4 1 6 3 9] | [2 4 1 7 6 9 5 8 2] | [2 3 6 4 7 1 8 5 2] | |
| [9 5 7 4 8 9] | [2 4 1 6 9 3 5 2] | [2 6 9 8 5 2] | |
| [2 6 3 9 7 4 1 8 5 2] | [2 3 9 4 1 7 6 8 5 2] | [2 3 9 8 2] | |
| [1 9 8 4 7 1] | [4 8 5 2 7 9 6 4] | [2 7 4 9 6 8 5 2] | |
| [2 4 8 7 1 3 6 9 5 2] | [3 6 5 8 2 7 4 9 1 3] | [2 6 9 7 4 1 5 2] | |
| [2 3 9 6 4 1 8 5 2] | [2 7 4 1 9 6 8 5 2] | [2 5 8 7 1 6 2] | |
| [1 8 9 7 4 3 1] | [2 3 6 7 9 5 8 2] | [1 9 5 7 4 1] | |
| [3 6 8 7 4 3] | [2 9 7 8 6 3 4 1 5 2] | [6 9 8 4 7 1 6] | |
| [2 3 6 4 9 5 2] | [2 4 1 3 9 7 6 8 5 2] | [3 9 8 5 7 4 3] | |
| [2 4 1 7 9 6 2] | [9 7 4 1 5 2 3 8 9] | [6 9 7 1 8 5 6] | |
| [2 3 8 5 4 1 2] | [2 7 4 8 5 2] | [2 3 6 4 1 8 9 5 2] | |

**Supplementary Figure 2: Representative Cluster Saccade Patterns for Monkey G.** The 136 identified saccade pattern clusters exhibited by Monkey G are shown in their numerical representations. The diagram at the top demonstrates how a saccade pattern is converted into a numerical representation. Each target on the grid is labeled as a number 1-9. The numerical representation of a pattern then follows to be the numerical sequence of target indices listed in the order that they would be visited when tracing out the pattern. Each cluster numerical sequence identifies the saccade pattern which was most similar to all other patterns in its cluster. The five most prominent clusters are marked by red type.

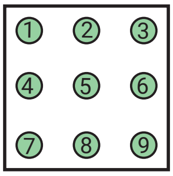


Grid Numbering

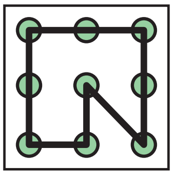

Example Pattern

**Example Numerical Representations**

(a) [1 3 6 9 5 8 7 1]

(b) [1 2 3 6 9 5 8 7 4 1]

(c) [1 3 9 5 8 7 1]

| #1-50 | #51-100 | #101-150 | #151-200 | #201-250 | #251-300 | #301-346 |
|---|---|---|---|---|---|---|
| [1 5 6 9 3 4 1] | [2 1 8 3 4 7 2] | [6 4 1 7 2 9 3 6] | [4 8 2 1 7 6 3 4] | [2 9 5 1 7 6 3 8 2] | [2 9 6 4 7 5 2] | [2 6 8 9 5 4 7 2] |
| [2 6 3 9 5 7 2] | [2 8 5 6 9 3 1 7 2] | [3 1 5 2 7 4 8 6 9 3] | [2 6 3 4 7 1 5 2] | [2 6 3 1 4 7 5 9 2] | [1 5 2 6 7 4 1] | [2 6 3 5 9 4 7 2] |
| [2 8 5 9 6 3 1 7 2] | [2 5 9 6 8 1 4 7 2] | [2 1 8 5 7 6 2] | [2 5 8 6 4 7 2] | [2 9 6 3 4 7 1 8 2] | [3 5 4 8 3] | [4 7 5 8 6 3 9 4] |
| [2 6 9 3 1 4 7 5 2] | [2 3 5 8 1 4 7 2] | [2 4 8 6 3 5 2] | [8 3 4 7 5 9 6 8] | [6 9 2 8 3 1 7 6] | [2 1 4 8 3 5 9 2] | [2 6 3 4 8 2] |
| [3 4 7 6 8 9 3] | [2 3 1 8 2] | [1 9 3 1] | [1 5 2 4 7 3 1] | [2 9 5 7 3 4 8 2] | [4 8 5 2 3 7 4] | [8 6 9 3 1 5 8] |
| [2 5 9 3 1 7 8 6 2] | [2 9 4 7 8 2] | [2 1 4 8 9 6 3 5 7 2] | [1 7 9 6 1] | [2 9 3 4 7 6 2] | [1 8 5 3 2 9 6 4 7 1] | [9 3 7 6 9] |
| [2 5 4 7 1 6 3 2] | [2 9 4 7 6 3 2] | [2 9 3 4 8 5 7 2] | [2 6 3 8 9 5 1 7 2] | [1 7 8 2 6 3 5 9 1] | [2 9 6 4 7 1 8 2] | [2 6 4 1 7 8 3 9 2] |
| [2 7 1 4 8 3 2] | [1 6 3 9 4 1] | [2 1 7 5 3 4 8 2] | [4 8 2 1 7 5 9 6 3 4] | [2 8 5 9 1 4 7 6 3 2] | [2 6 1 7 8 2] | [2 6 4 7 1 5 2] |
| [2 9 5 1 7 2] | [2 6 3 4 1 7 5 2] | [1 4 5 8 3 1] | [2 1 5 3 4 7 2] | [2 4 8 3 1 7 5 9 6 2] | [2 6 3 4 7 5 2] | [2 6 3 8 5 4 7 2] |
| [2 5 9 8 6 3 1 4 2] | [1 8 3 6 4 1] | [2 1 6 8 5 7 2] | [2 6 3 1 7 4 8 5 2] | [2 9 3 1 6 4 8 2] | [1 5 6 3 4 1] | [9 6 4 8 5 3 1 7 9] |
| [2 7 5 9 6 3 8 2] | [4 1 5 9 8 2 6 3 4] | [2 6 3 8 5 1 4 2] | [2 6 1 7 5 9 2] | [2 6 8 5 9 3 1 7 2] | **[2 1 7 9 6 3 8 2]** | [2 6 3 1 4 7 5 2] |
| [3 6 4 7 5 9 3] | [2 1 8 5 9 6 3 4 7 2] | [2 6 3 4 7 5 9 8 2] | [2 6 3 4 7 5 9 2] | [1 7 9 3 1] | [1 5 2 4 7 6 3 1] | [2 8 5 9 6 1 7 3 2] |
| [2 7 4 6 2] | [2 1 4 7 5 8 3 9 6 2] | [1 4 8 3 5 9 6 1] | [4 7 2 9 3 4] | [2 8 4 3 1 7 2] | [2 5 9 6 7 4 2] | [2 6 8 5 9 2] |
| [2 8 3 1 7 9 6 2] | [5 8 4 7 2 6 9 3 1 5] | [4 7 1 8 5 9 6 4] | [5 9 6 8 4 7 1 5] | [2 1 6 3 4 7 5 9 2] | [2 1 8 3 4 2] | [2 9 6 4 7 3 2] |
| [1 8 3 4 7 1] | [2 9 6 3 8 5 4 7 2] | [3 8 2 1 7 5 9 6 3] | [5 7 2 6 3 4 1 5] | [2 9 3 8 5 1 4 7 2] | [2 1 7 3 5 9 6 2] | [2 9 3 1 5 8 2] |
| [2 3 8 4 7 2] | [1 8 3 9 6 4 7 5 1] | [3 1 5 9 6 8 3] | [2 3 8 5 9 6 4 7 2] | [2 1 4 7 6 8 5 9 2] | [2 1 8 6 3 4 7 2] | [2 1 8 9 2] |
| [2 4 7 6 3 1 2] | [2 1 8 3 6 2] | [2 1 5 8 6 9 3 4 7 2] | [4 1 5 2 6 3 8 7 4] | [2 6 8 3 9 1 7 2] | [2 9 6 8 5 1 4 7 2] | [2 6 4 9 2] |
| [2 1 4 7 6 3 9 2] | [2 1 5 9 3 6 4 7 2] | [2 4 7 5 3 6 8 2] | [2 6 8 5 4 2] | [2 1 6 8 5 9 3 4 7 2] | [2 4 7 3 9 6 8 5 2] | [2 1 4 7 5 3 6 8 2] |
| [2 4 7 8 3 5 2] | [1 5 4 7 2 6 3 1] | [1 5 3 9 4 1] | [2 9 3 4 1 8 2] | [2 9 3 4 8 6 1 7 2] | [1 5 9 6 8 3 4 1] | [1 7 5 9 8 2 6 3 1] |
| [1 6 4 9 3 1] | [5 9 6 2 4 7 8 5] | [2 6 1 4 8 5 9 3 2] | [2 6 8 2] | [2 4 6 3 1 5 2] | [1 8 3 5 1] | [1 5 9 6 8 3 4 7 1] |
| [3 6 5 4 7 3] | [2 9 3 4 5 2] | [1 4 7 5 3 6 9 1] | [2 1 7 3 4 8 6 2] | [2 9 5 8 3 6 1 7 2] | [1 7 3 5 1] | [8 3 4 7 2 1 5 9 6 8] |
| [2 6 9 7 4 1 5 2] | [1 5 8 3 1] | [1 8 6 9 3 1] | [2 1 6 4 8 5 9 2] | **[2 5 3 6 2]** | [2 4 1 5 9 8 3 2] | [2 1 4 7 5 9 6 8 3 2] |
| [2 1 7 4 8 5 9 2] | [1 7 8 5 9 6 4 1] | [2 6 3 8 5 4 2] | [2 6 3 1 5 8 2] | [2 8 3 4 7 6 1 9 2] | [1 4 7 5 9 6 8 1] | [2 1 6 3 8 5 7 2] |
| [2 6 9 3 4 7 8 2] | [2 6 9 3 4 7 2] | [2 6 3 1 5 4 8 2] | [3 6 8 5 7 9 3] | [1 8 9 6 7 1] | [2 6 3 4 1 5 9 2] | [2 6 8 9 3 4 7 5 2] |
| [2 4 3 9 6 8 5 2] | [2 8 9 6 1 7 2] | [2 4 8 6 3 1 5 2] | [6 2 8 3 1 7 6] | [1 4 8 6 3 7 1] | [2 1 6 9 3 8 5 4 7 2] | [1 7 6 1] |
| [2 5 9 3 6 1 7 2] | [2 1 5 8 3 6 4 7 2] | [2 6 8 5 9 3 4 7 1 2] | [1 5 9 6 4 8 3 1] | [2 6 9 3 1 4 7 5 8 2] | [1 4 7 2 5 9 6 8 3 1] | [2 9 6 8 5 4 7 2] |
| [2 1 8 3 9 2] | [2 6 3 8 5 1 4 7 2] | [2 4 7 5 9 6 8 2] | [2 6 3 4 8 5 7 2] | [1 8 3 9 7 1] | [3 8 5 7 2 9 6 3] | [2 5 9 3 1 8 6 2] |
| [2 5 3 9 6 1 7 2] | [8 6 9 3 4 8] | [3 4 1 7 5 9 8 3] | [8 5 9 4 8] | [2 6 1 4 8 9 3 2] | [2 1 5 4 7 3 6 9 8 2] | [2 9 6 4 8 3 5 2] |
| [1 8 6 9 3 4 7 1] | [2 1 6 3 8 4 7 2] | [1 4 7 5 2 8 9 6 3 1] | [2 9 5 3 4 8 2] | [2 9 3 1 7 6 2] | [5 8 7 4 2 6 3 1 5] | [2 6 8 3 4 7 5 2] |
| [2 5 8 3 1 4 2] | [2 6 3 1 5 7 4 8 2] | [4 7 2 6 3 8 4] | [2 3 1 4 8 5 9 2] | [2 6 9 5 1 7 2] | **[1 5 8 6 3 1]** | [2 6 3 1 5 2] |
| [2 6 8 3 1 7 2] | [3 1 5 2 4 7 6 9 3] | [7 3 9 2 1 8 5 7] | [2 9 6 4 7 5 8 2] | [2 6 3 1 8 7 2] | [2 3 9 6 1 7 5 2] | [4 7 2 8 5 9 6 3 4] |
| [2 9 5 4 8 3 2] | [2 1 4 7 8 3 5 2] | [2 8 9 6 3 5 2] | [1 4 8 5 9 7 3 1] | [2 4 7 5 9 6 3 8 2] | [3 9 6 4 7 3] | [5 9 6 4 7 2 3 5] |
| [2 6 8 7 4 1 5 2] | [3 4 8 5 6 3] | [2 1 7 6 5 9 2] | [2 6 1 8 9 2] | **[6 3 4 1 5 9 6]** | [1 8 9 6 4 1] | [2 6 8 5 1 4 7 2] |
| [2 1 4 8 6 3 9 2] | [2 6 3 9 7 1 8 2] | [9 6 4 7 9] | [2 6 3 1 4 8 5 7 2] | [2 1 4 3 2] | [2 1 4 8 6 3 5 7 2] | [2 8 1 7 2] |
| [3 9 8 5 3] | [2 1 7 6 9 2] | [2 9 5 7 4 6 3 2] | [5 9 3 8 2 6 4 1 5] | [2 4 7 6 3 9 2] | [2 3 6 8 5 4 7 2] | [1 7 4 8 6 9 3 1] |
| [2 1 4 8 5 7 3 2] | [5 8 3 6 4 7 5] | [2 7 3 5 8 2] | [2 1 4 8 6 5 9 3 2] | [2 1 4 8 6 9 2] | [3 1 4 7 5 2 6 9 8 3] | [2 1 4 7 5 9 8 6 3 2] |
| [1 4 7 5 9 8 1] | [4 6 9 2 8 5 1 4] | [2 6 3 4 1 5 8 2] | [4 8 3 5 2 6 4] | [2 1 4 8 9 3 6 2] | [1 7 8 3 5 1] | [4 7 2 6 8 5 9 3 4] |
| [2 1 8 3 9 6 4 7 2] | [2 9 3 6 4 7 2] | [1 7 8 4 3 9 1] | [4 7 6 2 1 8 5 9 4] | [5 3 9 6 7 1 5] | [2 1 7 3 6 2] | [2 6 8 3 9 2] |
| [6 3 9 2 8 4 1 6] | [2 1 4 7 5 9 6 8 2] | [2 1 7 3 5 8 2] | [2 1 4 7 6 9 5 8 2] | [2 4 7 5 8 6 3 2] | [2 4 7 3 5 2] | [2 5 9 6 8 3 4 7 2] |
| [1 8 3 4 1] | [4 7 2 1 6 4] | [3 9 6 8 5 4 7 3] | [1 7 2 6 3 5 4 8 1] | [2 8 1 7 9 6 2] | [2 5 8 3 4 7 2] | [2 6 1 5 9 3 4 8 2] |
| [2 4 7 5 3 6 2] | [2 7 1 8 9 3 2] | [2 1 6 4 8 5 9 3 2] | [2 8 6 7 5 9 2] | [3 7 8 3] | [2 1 6 3 4 8 2] | [3 9 5 8 6 4 3] |
| [2 7 1 5 9 3 2] | [1 7 9 3 6 1] | [2 6 3 4 1 7 5 9 8 2] | [2 6 8 5 9 4 7 2] | [2 9 8 7 1 5 2] | [1 7 9 3 5 1] | [4 8 6 9 2 1 7 3 4] |
| **[2 4 7 6 3 5 2]** | [3 9 3] | [2 8 5 4 7 6 3 2] | [5 9 2 1 4 7 6 3 8 5] | [2 9 6 3 4 7 5 2] | [5 8 6 3 5] | [2 8 4 9 3 1 6 2] |
| [2 3 9 6 8 5 4 7 2] | [1 8 4 3 5 1] | [2 6 8 3 1 5 2] | [2 6 8 5 7 3 2] | [1 6 4 8 3 1] | [3 1 8 4 3] | [2 5 6 3 2] |
| [4 8 6 9 5 7 4] | [2 6 4 7 1 5 8 3 2] | [3 2 7 5 9 6 1 8 3] | [2 8 6 9 3 4 5 2] | [6 3 4 7 1 8 5 9 6] | [2 6 8 5 4 7 2] | [2 8 3 4 7 5 9 2] |
| [2 4 7 8 3 1 5 2] | [2 3 1 6 8 5 2] | [2 9 6 3 1 4 8 5 7 2] | [2 1 7 6 9 4 8 2] | [2 1 4 8 3 9 2] | [3 1 4 5 9 3] | [5 9 3 1 7 2 6 4 8 5] |
| [2 9 4 7 5 2] | [1 3 9 6 8 5 7 1] | [2 6 3 5 7 1 8 2] | [2 1 5 4 7 2] | [1 9 3 8 5 7 1] | [2 6 3 4 7 8 5 2] | |
| [2 6 1 4 8 3 2] | [2 6 8 9 3 1 7 2] | [2 9 6 4 7 5 8 3 2] | [2 1 5 9 3 4 7 6 8 2] | [5 1 4 7 2 3 9 6 8 5] | [1 8 6 9 3 4 7 5 1] | |
| [6 1 7 8 3 5 9 6] | [1 5 7 4 8 3 1] | [2 4 8 5 3 6 2] | [3 1 5 2 4 7 6 8 3] | [2 4 1 3 6 8 5 2] | [2 1 5 9 3 6 4 8 2] | |
| [2 1 7 8 5 6 3 9 2] | [4 7 2 5 8 9 6 4] | [2 6 8 7 4 3 5 2] | [2 8 9 3 1 6 2] | [2 6 8 5 3 1 4 7 2] | [2 1 9 3 4 7 2] | |

**Supplementary Figure 3: Representative Cluster Saccade Patterns for Monkey Y.** The 346 identified saccade pattern clusters exhibited by Monkey Y are shown in their numerical representations. The diagram at top demonstrates how a saccade pattern is converted into a numerical representation. Each target on the grid is labeled as a number 1-9. The numerical representation of a pattern then follows to be the numerical sequence of target indices listed in the order that they would be visited when tracing out the pattern. Each cluster numerical sequence identifies the saccade pattern which was most similar to all other patterns in its cluster. The five most prominent clusters are marked by red type.

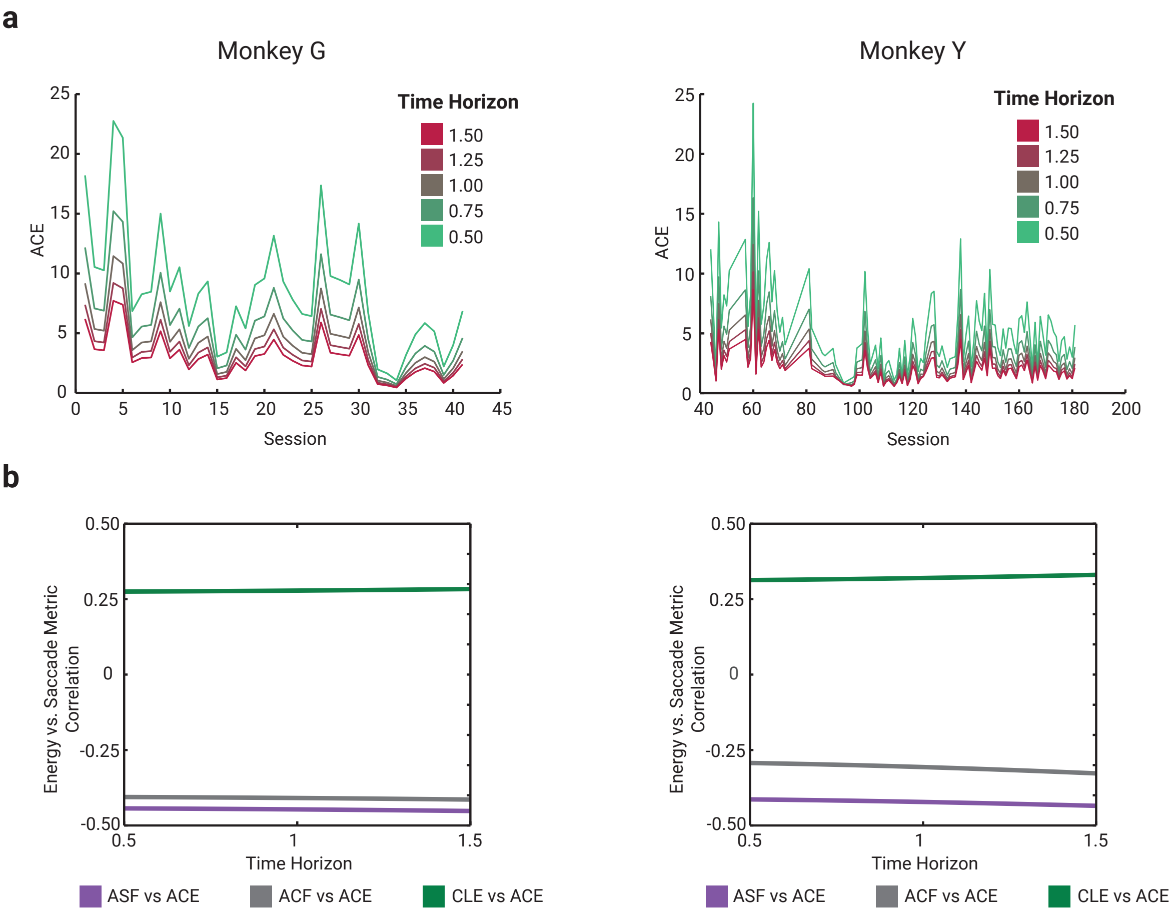


**Supplementary Figure 4: Control Energy Dynamics: Time Horizon Parameter Sweep.** **(a)** Average control energy dynamics across all sessions for Monkey G (left) and Monkey Y (right) using five different values of the time horizon parameter. Smaller time horizon values result in higher magnitude energy values and *vice versa*. The time horizon was set to a value of 1 for all analysis in the main text. **(b)** All three energy-behavior correlations were re-calculated using the control energy derived from a range of time horizons (0.5 to 1.5 in intervals of 0.1). The change in each energy to behavior (average similarity factor, average complexity factor, and cluster label entropy) correlation is shown as a function of the time horizon (Monkey G - Left; Monkey Y - Right).

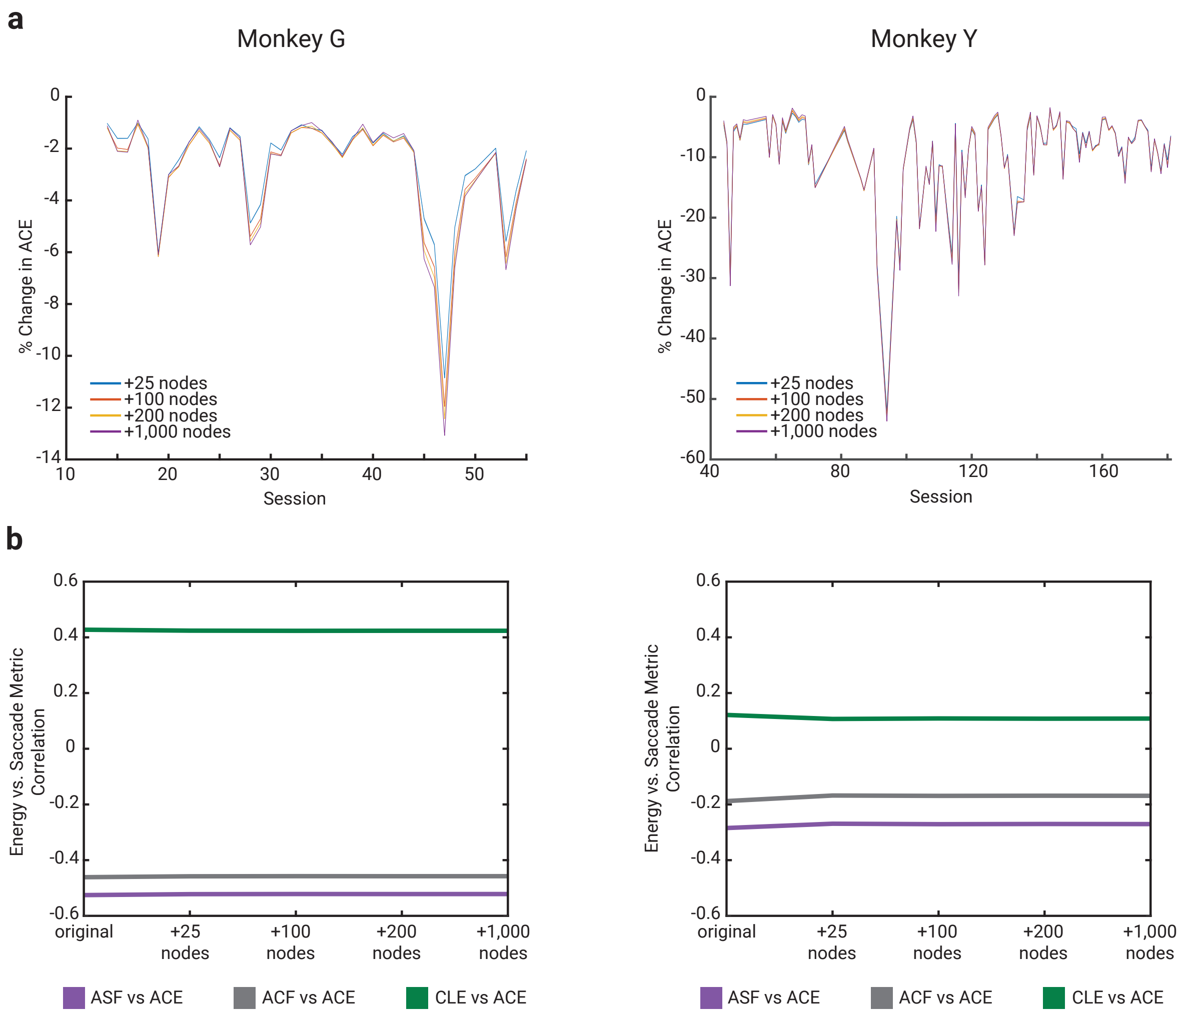


**Supplementary Figure 5: Control Energy Dynamics: Sub-Graph Sampling Simulation.** **(a)** Percent change in average control energy across all sessions for Monkey G (left) and Monkey Y (right) after simulation of networks containing 25, 100, 200, or 1,000 additional nodes (mean +/- SEM for 10 networks of each size). In each simulation, control input is given only to regions present in the original network, such that the B matrix contains ones along the diagonal of the original circuit regions and zeros elsewhere. The percent change in control energy induced by adding nodes to the network does not vary as a function of network size. The relationship between ACE and session is preserved across all network sizes (there is a correlation of $r \geq 0.999$ between the control energy across sessions for the original network and the corresponding values for each expanded network). **(b)** All three energy-behavior correlations (uncorrected for number of channels) were re-calculated using the control energy derived from networks containing 25, 100, 200, or 1,000 additional nodes. The change in each energy to behavior (average similarity factor, average complexity factor, and cluster label entropy) correlation is shown as a function of network size (Monkey G - Left; Monkey Y - Right).

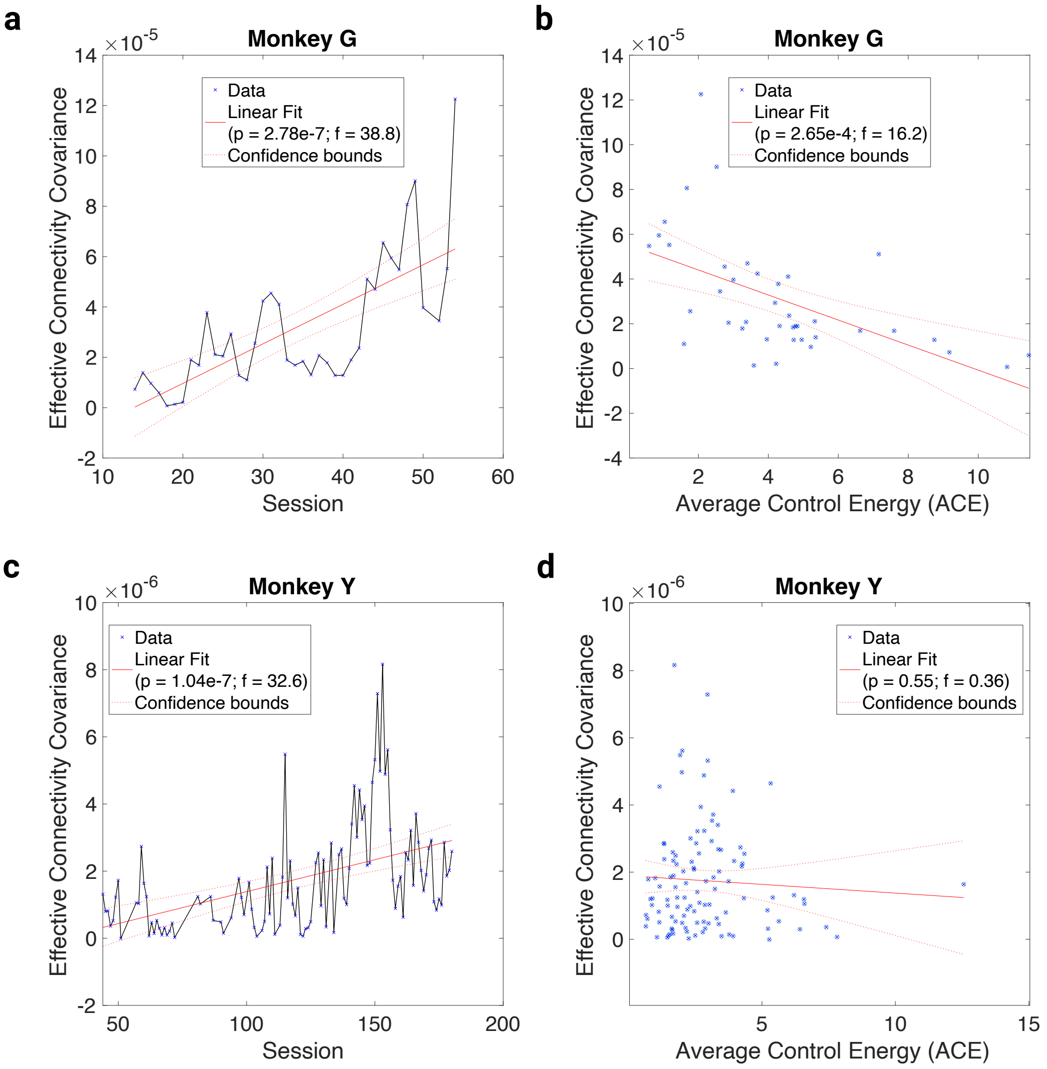


**Supplementary Figure 6: Session Effective Connectivity Variability Changes.** **(a,c)** Covariance between the session effective connectivity matrices across successive sessions were plotted across session IDs, for Monkey G and Monkey Y. For both monkeys, EC covariance appears to significantly increase with session count (Monkey X: $p_{value} = 2.78\text{e-}7$; $f_{statistic} = 38.8$; sub-plot **(a)** and Monkey Y: $p_{value} = 1.04\text{e-}7$; $f_{statistic} = 32.6$; sub-plot **(c)**.) **(b,d)** Covariance between the Effective Connectivity matrices across successive sessions was also plotted versus Average Control Energy, in both monkeys. There was a significant negative correlation between the two metrics for Monkey G ($p_{value} = 2.65\text{e-}4$; $f_{statistic} = 16.2$; sub-plot **(b)**), but not for Monkey Y ($p_{value} = 0.55$; $f_{statistic} = 0.36$; sub-plot **(d)**).

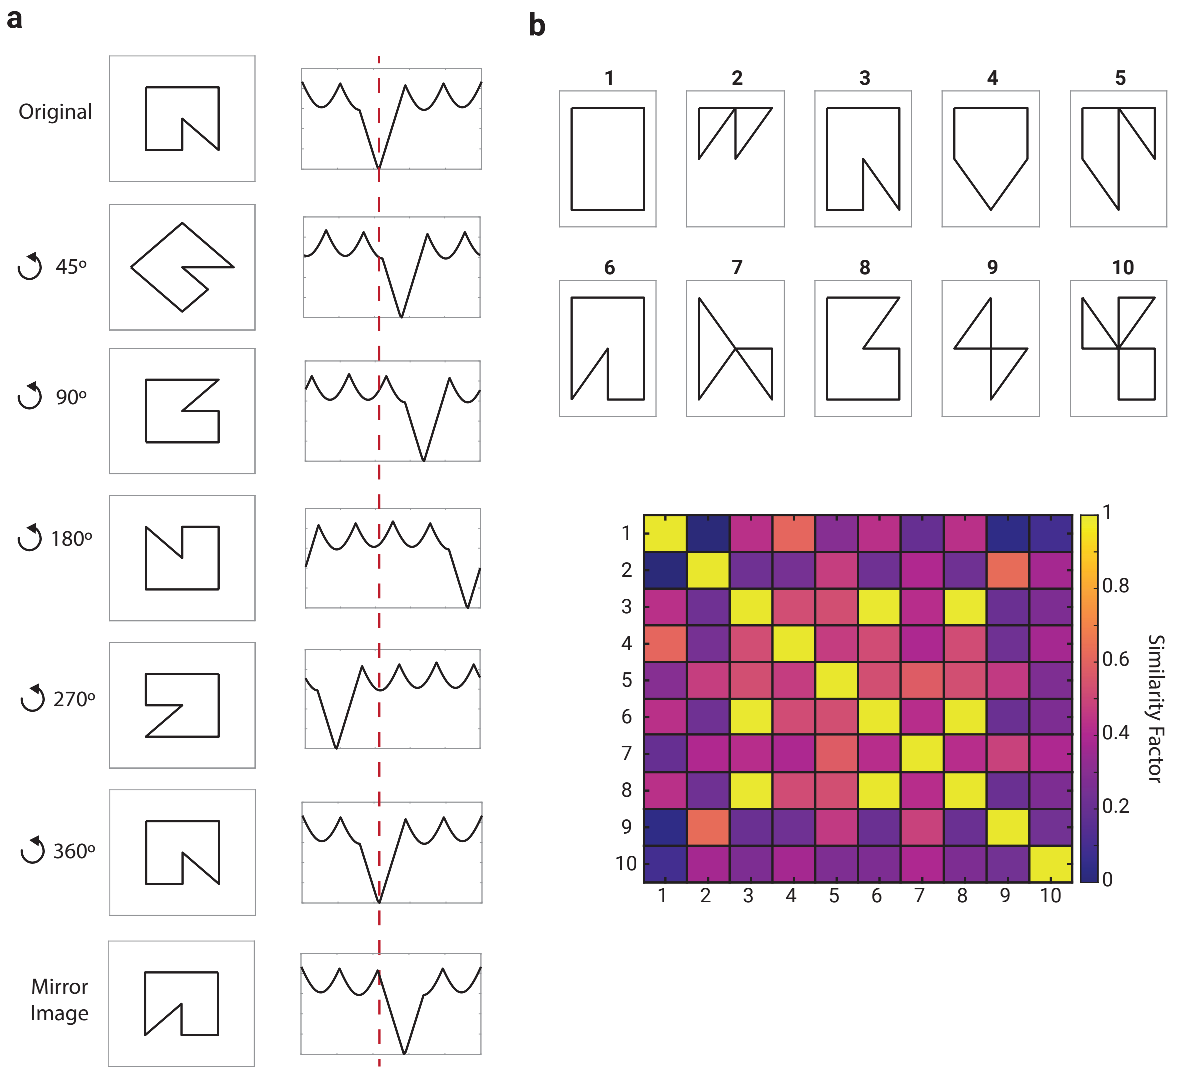


**Supplementary Figure 7: Rotational Independence of the Similarity Factor**. The similarity factor metric to compare saccade patterns from trial to trial was designed to be independent of rotation. **(a)** Performing circular shifts to the saccade waveform is equivalent to rotation of the saccade polygon. A circular shift is a mathematical operation where a vector is rearranged such that the last element is moved to the first position and all other elements are shifted forward by one. By performing this operation $l$ times, it is possible to shift the last $l$ values to the front of the vector and all other values forward by $l$ positions. This relationship is depicted as the pattern rotates counter clockwise, the waveform shifts all elements forward. In addition, the mirror image of the original polygon can be represented by flipping the original saccade waveform left-to-right. The red-dashed line is meant to serve as a visual aid. **(b)** Ten arbitrary saccade patterns and their calculated similarity matrix. The rotational independence of the measurement is evident as the value of similarity between pattern 8 and patterns 3 and 8 is equal to 1 (the highest value). Note that the value of similarity between pattern 6 and 3 (direct mirror images) is also equal to 1.

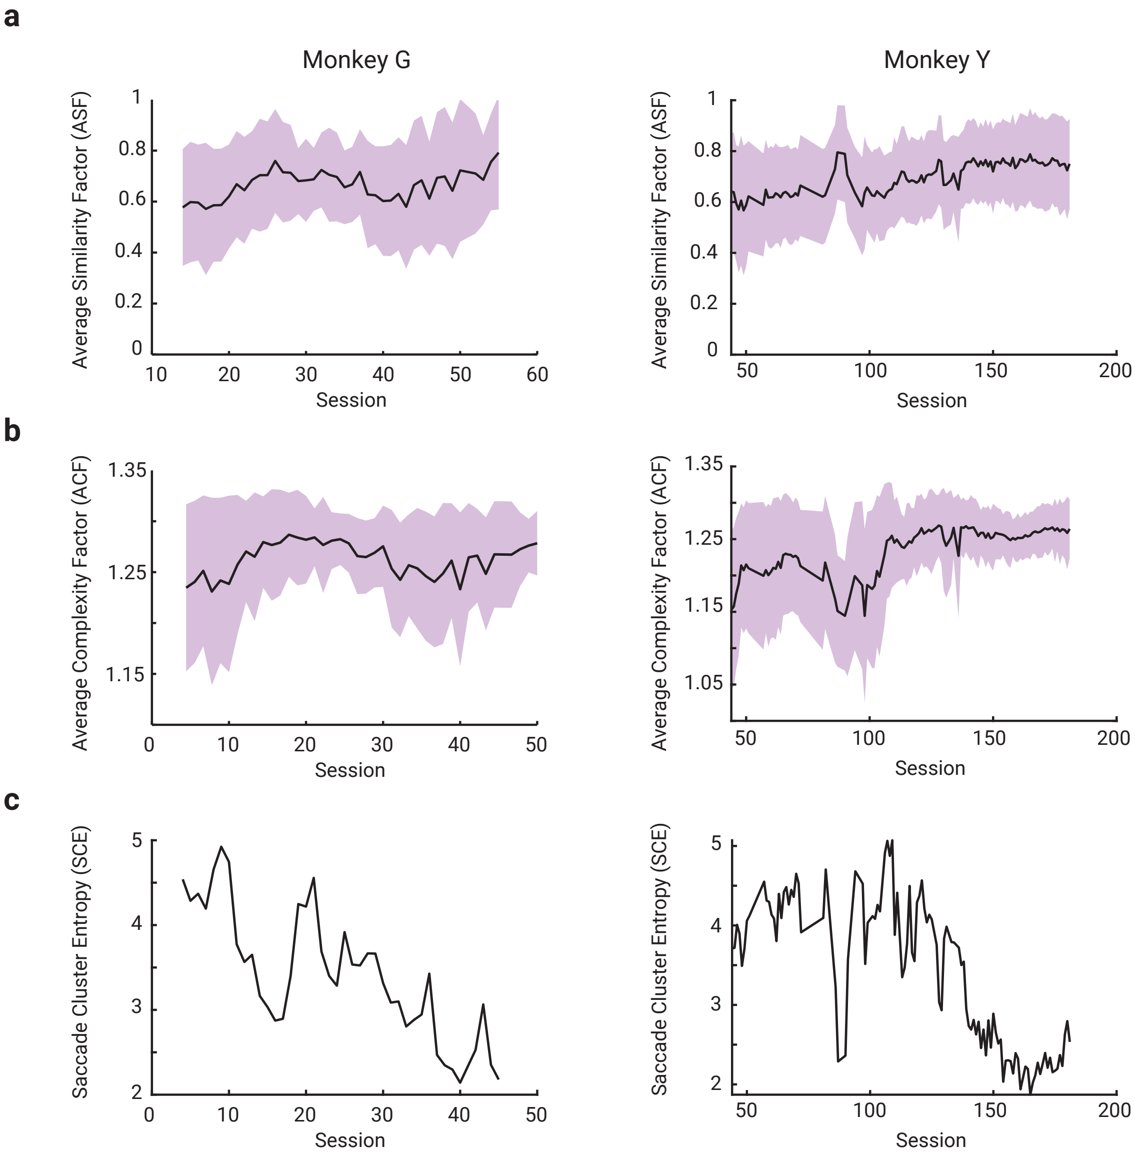


**Supplementary Figure 8: Saccade Metric Dynamics**. **(a)** Dynamics of the average similarity factor across all sessions for Monkey G (Left) and Monkey Y (Right). Filled boundary areas represent +/- 1 standard deviation. **(b)** Dynamics of the average complexity factor across all sessions for Monkey G (Left) and Monkey Y (Right). Filled boundary areas represent +/- 1 standard deviation. **(c)** Dynamics of the cluster label entropy across all sessions for Monkey G (Left) and Monkey Y (Right).

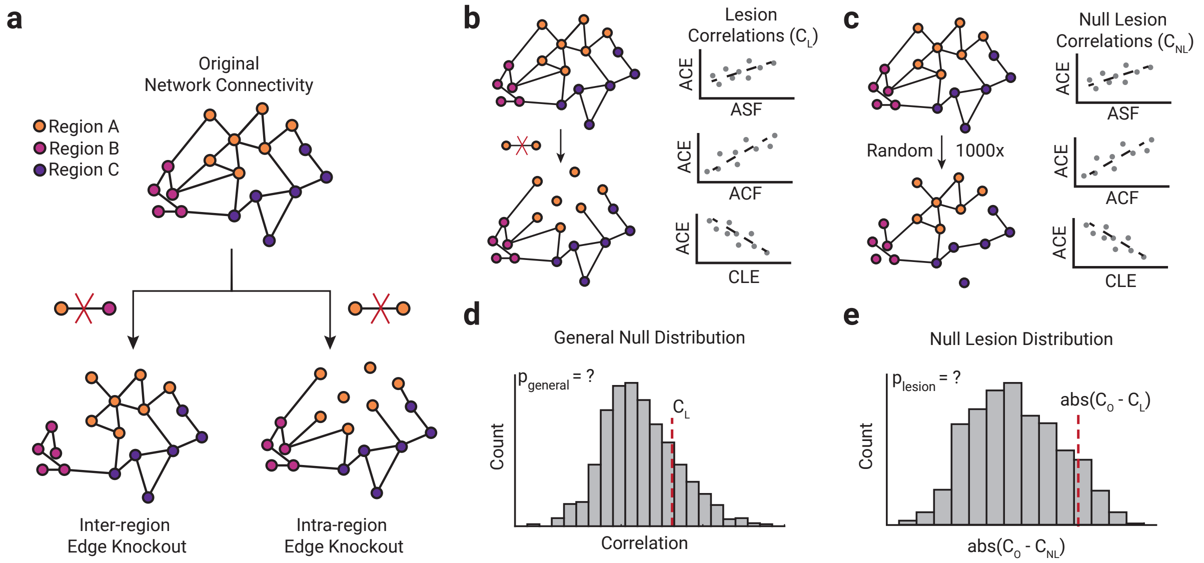


**Supplementary Figure 9: Virtual Region Specific Lesion Analysis Guide**. **(a)** Visual depiction of the lesion analysis workflow. The lesion knockout consists of performing a series of edge-knockouts where (i) all edges between two regions are set to zero in the effective connectivity matrix (inter-region), or where (ii) all edges connecting one region to itself are set to zero (intra-region). **(b)** For each region specific lesion, the effective connectivity matrix with region specific edges knocked out is used to compute the average control energy and its correlation ($C_L$) to the saccade metrics. **(c)** Random lesions (1000x) were performed to ensure that the lesion-induced disruption of the observed correlations between average control energy and the behavioral metrics was specific to the lesion chosen, and not expected by lesioning the same number of randomly chosen edges. For each random lesion the average control energy and its correlation ($C_{NL}$) to the saccade metrics was computed. **(d)** The first criterion to test whether the knockout edges were relevant to the observed energy-behavior correlations, was that the region specific lesion resulted in a lesion correlation value, $C_L$, that was not significantly different ($p > 0.05$) from that obtained using the original permutation null model. The obtained $p$-value from such a significance test is referred to as, $p_{general}$. **(e)** For the second criterion, a null lesion distribution was created with each value being calculated as the $abs(C_O - C_{NL})$, where $C_O$ is the observed energy-behavior correlation without any lesions. The significance of the region specific lesion disruption ($abs(C_O - C_L)$) of the observed correlations was determined using a one-tailed test on the null lesion distribution with $\alpha = 0.05$. The obtained $p$-value from such a significance test is referred to as, $p_{lesion}$.

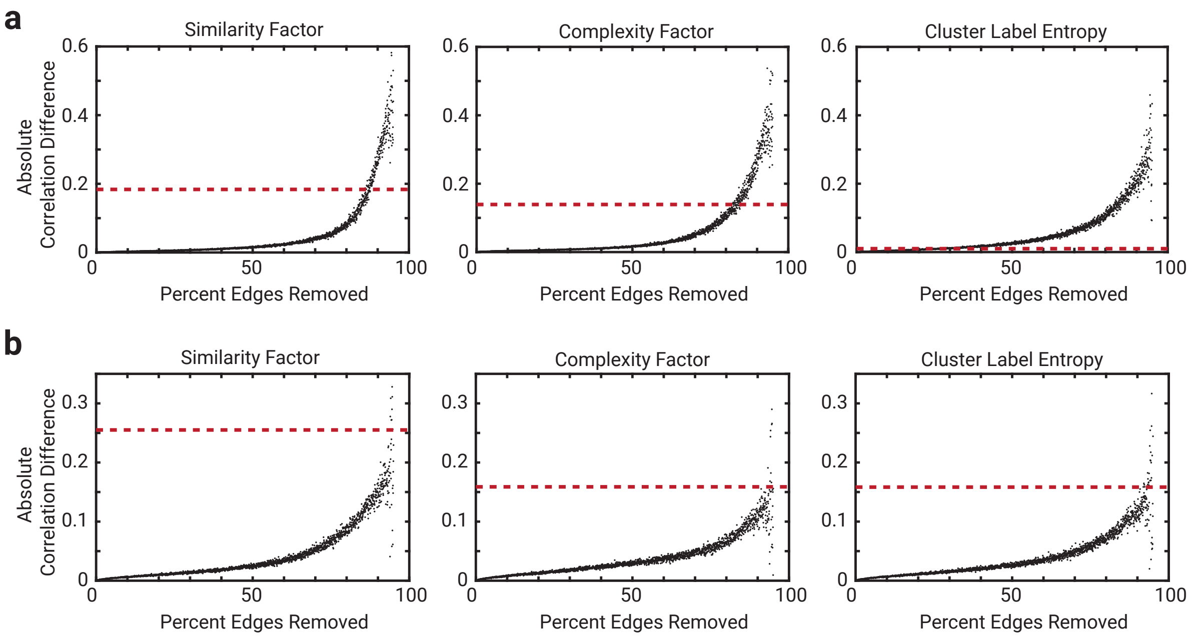


**Supplementary Figure 10: Resilience of Energy-Behavior Correlations to Network Disruption**. **(a-b)** Resilience of energy-behavior correlations as a function of number of edges randomly lesioned for Monkey G **(a)** and Monkey Y **(b)**. Every lesion was performed 100 times and each plot value is therefore the average absolute correlation difference. The absolute correlation difference was calculated as the difference between the observed energy-behavior correlation without any lesioning and the correlation after random edges were lesioned from the effective connectivity matrix. Red dashed lines denote the minimum threshold required to significantly disrupt the energy-behavior correlation such that its $p$-value is greater than $\alpha = 0.05$. ACE: Average Control Energy, ASF: Average Similarity Factor, ACF: Average Complexity Factor, CLE: Cluster Label Entropy.

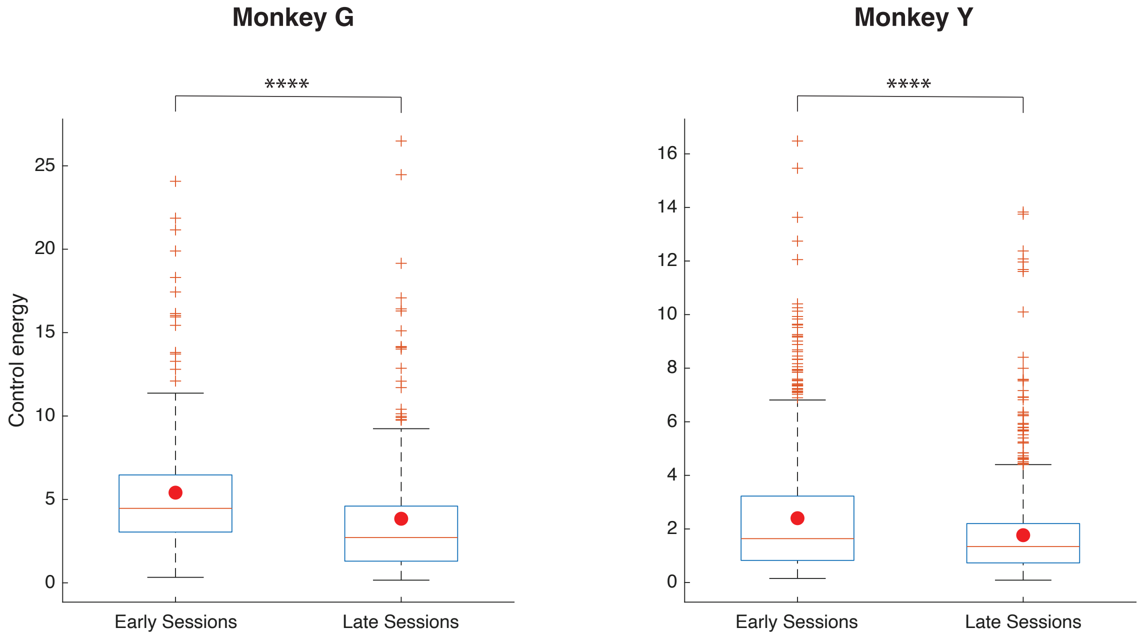


**Supplementary Figure 11: Energy Cost associated with Transitioning between Equally Complex Behavioral Strategies in Early versus Late Sessions**. For both MG (left) and MY (right), the energy cost associated with transitioning between behavioral sequences of the same complexity factor is lower, on average, in later sessions as compared to earlier sessions (****$p < 0.0001$). For each unique transition type, energy values were averaged across all instances within early sessions and within late sessions, so that each transition contributed a single value per epoch. Reported $t$-tests are therefore based on the number of unique transition types observed in both early and late epochs. "Early Sessions" include the first half of all sessions analyzed in this study, and "Late Sessions" include the second half. The box plots show the median (horizontal line), interquartile range (box), and range excluding outliers (whiskers). The red dots indicate the mean for each group.

# Supplementary Analysis 1

### Is the centroid measure utilized in the comparison of saccades robust to noise?

In this section, we examined whether the centroid measure utilized in saccade comparisons was robust to noise. Specifically, for each trial's TRSP sequence, we randomly selected a node and displaced it to a random position within a circle whose center was the node's original position and whose radius was set to a value $r$. Because each node was on a grid, we picked $r = 0.1$ and $r = 0.2$ as two representative radii to model noise. After generating the new centroids corresponding to each 'noisy' TRSP sequence, we generated three vectors: one corresponding to the list of centroids obtained from the original TRSP sequences, one corresponding to the centroids obtained from the new slightly 'noisy' TRSP sequences (with $r = 0.1$), and one corresponding to the centroids obtained from the more 'noisy' TRSP sequences (with $r = 0.2$). We performed a two-sample *t-test* across each combination of these three vectors, yielding distributions that were highly similar to each other (Monkey G: original centroids versus 10 percent noise: $p = 0.99$; original centroids versus 20 percent noise: $p = 0.99$; 10 percent noise versus 20 percent noise: $p = 1$). We can thus deduce that our centroid measure utilized in the comparison of saccades was robust to reasonable amounts of added noise.

# Supplementary Analysis 2

### Is there a 1:1 relationship between saccade paths and their centroids?

To address this question, we constructed the TRSP corresponding to each trial, for each session, and for each monkey, and examined whether there were any two TRSPs giving rise to the same centroid. For Monkey G, out of the 9,702 TRSPs (and their corresponding centroids), there were 324 centroids that were repeated more than once. For Monkey Y, out of the 80,664 TRSPs (and their corresponding centroids), there were 983 centroids that were repeated more than once. For each repeated centroid, we investigated whether it was the same TRSP that was giving rise to the same centroid, or whether there were different TRSPs giving rise to the same centroid. We established that for both monkeys there was a 1:1 relationship between TRSPs and their centroids, and that every time a centroid was repeated across two different trials it was because the TRSP sequence between these two trials was also the same.

# Supplementary Analysis 3

**Is there bias introduced by utilizing the same spikes (i.e., firing patterns) to infer effective connectivity and the average minimum control energy (ACE) across sessions?**

To investigate whether there is a potential circularity issue in our results—in that spikes used to infer the effective connectivity matrices are among those used to also estimate the control energy, we performed the following analyses:

We first inferred the effective connectivity matrix from each session based on the first half of their respective trials (i.e., floor function of the total number of trials for each session divided by two); the overall effective connectivity matrix across all sessions (denoted here as $A_{updated}$) was then computed as the average of all sessions' effective connectivity matrices. Next, we calculated the ACE of each session using only the spiking information from the remaining trials (i.e., the trials that were not used to infer the effective connectivity matrices). In other words, we used the second half of the trials to define our initial and target states (as defined in equations 6 and 7 in the text) to compute each session's new ACE. Given that we need the effective connectivity matrix to compute the ACE, we used $A_{updated}$ for this calculation. After performing this analysis, we were able to generate new ACE values for each session.

To examine whether these newly-derived ACE values differed from our empirically-derived (original) ACE values reported in the manuscript, we performed the following two statistical comparisons:

A) A two-way Kolmogorov-Smirnov test (*kstest2* command in MATLAB) to examine whether the empirically-derived ACE and the newly-derived ACE vectors could be part of the same distribution. Indeed, both vectors were found to be part of the same distribution for both monkeys (Monkey G: $ks_{stat} = 0.0732$, $p = 0.9999$; Monkey Y: $ks_{stat} = 0.0636$, $p = 0.9751$).

B) Next, we repeated the linear correlations between ACE and the three saccade characteristic metrics (average similarity factor [ASF], average complexity factor [ACF], and cluster label entropy [CLE]), shown in Figures 5e and f in the main manuscript, using the newly acquired ACE values. The results were virtually identical to the ones reported in the manuscript, using the empirically-derived ACE values, for both monkeys (Monkey G: ACE vs ASF: $R^2 = 0.175$, $p = 0.0065$, ACE vs ACF: $R^2 = 0.163$, $p = 0.0089$, ACE vs CLE: $R^2 = 0.069$, $p = 0.0979$; Monkey Y: ACE vs ASF: $R^2 = 0.168$, $p = 8.58 \times 10^{-6}$, ACE vs ACF: $R^2 = 0.081$, $p = 0.0027$, ACE vs CLE: $R^2 = 0.096$, $p = 0.001$; adjusting for

number of channels).

Both of these results indicate that there was no (significant) circularity issue introduced by using the same spikes to infer the effective connectivity matrices and estimating control energy.
